# Supplementary material for: Mobile Foundation Model as Firmware
Source: arXiv:2308.14363 source file (2024-03-12)
Supplement: Supplementary file 1 [file sec-appendix.tex]

\section*{Appendix} \label{sec:appendix}

\input{sec-appendix-models.tex}
